# Supplementary material for: Shuffle and Joint Differential Privacy for Generalized Linear Contextual Bandits
Source: arXiv:2602.00417 source file (2026-04-27)
Supplement: Supplementary file 1 [file appendix_regret_lm_proof.tex]

\section{Proof of Theorem \ref{thm:general_regret_guarantee}}{\label{sec:main_theorem_linear_contextual}}

% The privacy analysis of the shuffle convex optimizer $\mathcal{P}_{\text{GD}}$ directly follows from \cref{lemma:elimination_first_step} which uses the advanced composition theorem \cite{dworkdpbook}. The privacy analysis of the vector summation protocol  follows from \cite[Theorem 4.2]{Cheu2021ShufflePS} which can be shown to be $(\varepsilon/2, \delta/2 - \frac{1}{T^2})$ shuffle differentially private conditioned on the event $\frac{\dot{\mu}(\langle x_t, \hat \theta_1\rangle)}{\beta(x_t)} \leq \frac{1}{\kappa^{*}}$. Further, since this event holds with probability at least $1-\frac{1}{T^2}$, the desired $(\varepsilon,\delta)$ shuffle differential privacy holds for estimators $\tV \text{ and } \{\tH_k\}_{k \geq 2}$.

Since, the set of estimators $\{\hat \theta_k\}_{k=1}^{M}, \tV \text{ and } \{\tH_k\}_{k \geq 2}$ are $(\varepsilon,\delta)$ differentially private with the data $\{r_t,\gX_t\}$ in the $k^{th}$ batch, the desired $(\varepsilon,\delta)$ multi-rounded shuffled privacy guarantee naturally follows. Further, we can show that this algorithm naturally satisfied JDP via \cite[Billiboard's lemma]{mechanism_design_large_games}.

\begin{proof}
 Fix any batch $k$ such that $k \geq 2$, when conditioned on the first $(k-1)$ batches, we let $\gD_k$ be the distribution of the survived candidate arms $\mathcal{X}^{(k)}_t$ at any time $t$ during the $k$-th batch. We also let $\gD_0$ denote the distribution of all candidate arms at any time $t$.

Suppose that the desired event in \cref{lemma:conf} happens for every time step during the $k$-th batch (which happens with probability at least $(1 - \delta B_k/T^2)$ by a union bound), it is straightforward to verify that for each time $t$ during the $k$-th batch, the optimal arm is not eliminated by the elimination procedure Line \ref{line:lm_elimination}. In other words, we have that $x^{*}_t \defeq \argmax_{x \in \gX} x^\top \theta$ for each time step $t$ in the $k$-th batch. 

Further, we define the $\omega_{x}^{(k)} = \alpha \sqrt{x^{\top} \mLambda_{k}x}$ as the confidence bounds for arm $x$ as defined in \cref{eq:confidence_bounds}. Therefore, we can now upper bound the expected regret incurred during batch $k$ as 
\begin{align}
R_k & = \E \sum_{t \text{~in batch $k$}} (\max_{x \in \gX_T} x^\top \theta - x_{t}^\top \theta) 
 \leq  \E \sum_{t \in \gB_k} (\langle x^{*}_t \hat{\theta}_{k-1} \rangle- x^\top \hat{\theta}_{k-1} + \omega_{x}^{(k-1)} + \omega_{x}^{(k-1)}) \label{eq:thm-blinucb-10}\\
& \leq  \E \sum_{t \in \gB_k}  2 \cdot (\omega_{x}^{(k-1)} + \omega_{x}^{(k-1)}) \leq 4 \E \sum_{t \in \gB_k} \max_{x \in \mathcal{X}^{(k)}_t} \omega_{x}^{(k-1)} , \label{eq:thm-blinucb-20}
\end{align}
where \eqref{eq:thm-blinucb-10} is due to the successful events of \cref{lemma:conf}, the both inequalities in \cref{eq:thm-blinucb-20} are due to the elimination process and that $x_t^{*} \in \gX^{(s)}_t$. By the definition of $\omega_{x}^{(k-1)}$ and the definition of $\gD_k$, we further have that
\begin{align} 
R_k\leq 4\alpha \E\sum_{t \text{~in batch $k$}} \max_{x \in \gX^{(s)}_t} \sqrt{x^\top \mLambda_{k-1}^{-1} x}  \leq 4\alpha \times \sum_{t \text{~in batch $k$}} \E_{\gX \sim \gD_{k}}\max_{x \in \gX} \sqrt{x^\top \mLambda_{k-1}^{-1} x}.  \label{eq:thm-blinucb-30}
\end{align}
We finally observe that $\gX \sim \gD_k$ can be sampled by drawing an $\gX' \sim \gD_{k-1}$ and performing an elimination process using $\hat\theta_{k-1}$ as well as the corresponding confidence region for $\gX'$. We note that $\gX \subseteq \gX'$. Therefore, continuing with \eqref{eq:thm-blinucb-30}, we have that
\begin{align}
R_k \leq 4\alpha \times \sum_{t \in \gB_k} \E_{\gX \sim \gD_{k-1}}\max_{x \in \gX} \sqrt{x^\top \mLambda_{k-1}^{-1} x} = 4\alpha \gT_k \times \E_{\gX \sim \gD_{k-1}}\max_{x \in \gX} \sqrt{x^\top \mLambda_{k-1}^{-1} x}. \label{eq:thm-blinucb-40}
\end{align}

% Now the goal is to upper bound $\E_{X \sim \gD_{k-1}}\max_{x \in X} \sqrt{x^\top \mLambda_{k-1}^{-1} x}$. The following lemma is a direct application of  %\autoref{lem:conconcut}  in \appref{app:concentration}.

Assuming that \eqref{eq:lem-exploration} holds for batch $(k-1)$, letting $x^*(\gX) = \argmax_{x \in \gX} x^\top \mLambda_{k-1}^{-1} x$, we have that
\begin{align}
&  \E_{\gX \sim \gD_{k-1}}\max_{x \in \gX} \sqrt{x^\top \mLambda_{k-1}^{-1} x}  = \E_{\gX \sim \gD_{k-1}} \sqrt{(x^*(\gX))^\top \mLambda_{k-1}^{-1} x^*(\gX)} \nonumber \\
&\qquad \qquad \leq  \sqrt{\E_{\gX \sim \gD_{k-1}} (x^*(\gX))^\top \mLambda_{k-1}^{-1} x^*(\gX)} = \sqrt{\Tr(\mLambda_{k-1}^{-1} \E_{\gX \sim \gD_{k-1}}  x^*(\gX) (x^*(\gX))^\top)},
 \label{eq:blinucbkw-1800}
\end{align}
where the inequality is by Jensen's inequality. By \cref{eq:thm-KW} (up to the factor $2$ relaxation), we have that 
\begin{align}
 x^*(\gX) (x^*(\gX))^\top \preceq 2d \times \E_{\vy \sim \gopt(X)} \vy\vy^\top . \label{eq:blinucbkw-1900}
\end{align}
Combining \eqref{eq:blinucbkw-1800} and  \eqref{eq:blinucbkw-1900}, we have that
\begin{align}
\E_{\gX \sim \gD_{k-1}}\max_{x \in \gX} \sqrt{x^\top \mLambda_{k-1}^{-1} x} \leq \sqrt{2d \times \Tr(\mLambda_{k-1}^{-1} \E_{\gX \sim \gD_{k-1}}  \E_{y \sim \gopt(\gX)} yy^\top )} \leq 4\sqrt{2} d/ \sqrt{\gT_{k-1}},\label{eq:blinucbkw-2000}
\end{align}
where the last inequality is due to \eqref{eq:lem-exploration}. Combining \eqref{eq:blinucbkw-2000} and \eqref{eq:thm-blinucb-40}, we have that with probability at least  $(1 - 2\gT_k/T^6)$, the expected regret incurred during batch $k$ ($k \geq 2$) is
\begin{align*}
R_k \leq 4\alpha \gT_k \cdot  4\sqrt{2}d / \sqrt{\gT_{k-1}} \leq 16\sqrt{2} \alpha d\sqrt{T}. %\label{eq:thm-blinucbkw-2100}
\end{align*}

One should observe that the expectation is over the randomness in the generation of the contexts $\gX_t$ in the $k^{th}$
batch while the high probability guarantee is over the randomness in all previous batches which includes randomness in user's noise addition mechanism and the sampling of the arms from the context set.

Thus, the expected regret may be bounded as $R^T = \sum_{k \in [M]} (R_k + \frac{1}{T^4} T) = O(d \alpha \sqrt{T} \log \log T).$

% Thus, summing over all batches, we can compute the cumulative regret as $\tilde{O}(1/\varepsilon \sqrt{T})$

\end{proof}
